# Supplementary material for: InternVLA-M1: A Spatially Guided Vision-Language-Action Framework for Generalist Robot Policy
Source: arXiv:2510.13778 source file (2025-10-15)
Supplement: Supplementary file 1 [file D_long_tasks.tex]

\section{ xxx xxx xxx}
Beyond evaluating our model's generalization in single-step pick-and-place instruction following, we also assess its robustness in long-horizon tasks that require dynamic task planning, re-planning under instruction or environmental changes, and complex multi-stage reasoning. Specifically, we design three challenging interactive tasks to probe these capabilities:

\noindent\textbf{Math calculation.} \yilun{@fangjing, add goods purchase} The robot is given an arithmetic equation and must compute the correct solution. It then compares this result with a set of candidate options, each uniquely associated with a specific color. Once the matching option is identified, the robot maps the answer to its corresponding color cue and presses the designated button.

\noindent\textbf{Desktop sorting.} The robot is instructed to sort objects into containers based on high-level category descriptions. There are five object categories—\textit{fruits, toys, vegetables, bottles}, and \textit{snacks}—and each task instance involves sorting objects from one to three categories into their respective target containers.

\noindent\textbf{Sorting items into drawers.} The robot must sequentially (i) open a designated drawer, (ii) place the specified objects into it, and (iii) close the drawer, requiring precise temporal reasoning and articulated object manipulation.

\noindent\textbf{Making sandwiches.} The robot is required to assemble a sandwich according to a provided meal recipe. Each episode begins with two slices of bread, two slices of meat, and two leaves of lettuce on the table. The robot must place the ingredients in a specific order (bread → meat → lettuce → bread) onto a plate to construct one of five predefined sandwich types.

\begin{figure}[ht!]
    \centering
    \includegraphics[width=1.\textwidth]{figures/real-world-tasks-showcase.pdf}
    \caption{Showcase for long-horizon instruction-following manipulation.}
    \label{fig:real-world-long-horizion-showcase}
\end{figure}

To support fine-grained training for these long-horizon tasks, we collect a total of \textbf{22 hours} of high-quality teleoperated demonstrations, amounting to approximately 400–500 trajectories per task. Each collected trajectory is segmented into \textit{subtasks} and annotated with corresponding atomic actions. For example, a “make a classic sandwich” task is decomposed into four subtasks:
(1) “Put a piece of bun on the plate.” →
(2) “Put a piece of meat on the plate.” →
(3) “Put a piece of lettuce on the plate.” →
(4) “Put a piece of bun on the plate.”
Each sub-instruction is paired with a specific segment of the demonstration.
To enable subtask-level grounding and transition, we introduce padding (zero-action vectors) after each subtask segment to signal task completion and prompt the model to predict and transition to the next subtask. Additionally, to enhance temporal consistency and model inference smoothness, we remove frames where the robotic arm exhibits clear pauses or idle behavior.

Similar to the short-horizon instruction following evaluation, we also assess the performance of our model on these three long-horizon tasks under the \textbf{in-distribution (ID)} setting, where all objects involved in the tasks—whether for desktop sorting, drawer cleanup, or sandwich assembly—are drawn from categories and instances seen during training.
In addition to this, we evaluate the model’s capability to \textit{re-plan and re-act} in the presence of dynamic changes to the environment or instructions. Specifically, we introduce perturbations such as changes in the object layout, container positions, drawer states, or alterations in the instruction formulation (e.g., switching from direct commands to attribute-based or goal-conditioned prompts). This setup probes the model’s ability to adjust plans mid-execution, recover from disruptions, and continue progressing toward task completion with stability and reliability.
